# Supplementary material for: On the surface chemisorption of oxidizing fine iron particles: insights gained from molecular dynamics simulations
Source: arXiv:2212.06432 source file (2023-04-19)
Supplement: Supplementary file 1 [file Init_velocities.tex]

\section{Incident velocities}\label{sec:incident_Vel}
The diatomic molecule is modelled as rigid rotaters, where the initial velocity of each atom is prescribed. Figure \ref{fig:RigidRotor} shows a schematic representation of the diatomic nitrogen molecule.
\begin{figure}[h]
    \centering
    {\includegraphics[width=0.5\columnwidth]{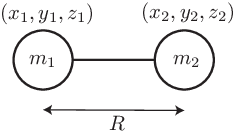}}
    \caption{Schematic representation of the diatomic nitrogen molecule represented as a rigid rotor}%
     \label{fig:RigidRotor}
\end{figure}

The translational energies of the molecule are sampled from the flux-corrected Maxwell-Boltzmann (MB) distribution, where the three velocities are described via \citep{Mane2018}
\begin{equation} \label{eq:mb_vxy}
    f\left(v_{CoM,x,y}\right) = \left( \frac{\bar{m}}{2\pi k_\mathrm{B} T} \right)^{1/2} \exp{\left(\frac{- \bar{m} v_{CoM,x,y}^2}{2 k_\mathrm{B} T} \right)},
\end{equation}
\begin{equation} \label{eq:mb_vz}
    f\left(v_{CoM, z}\right) = \left( \frac{\bar{m}}{k_\mathrm{B} T} \right)^{1/2} v_{CoM,z} \exp{\left(\frac{- \bar{m} v_{CoM,z}^2}{2 k_\mathrm{B} T} \right)},
\end{equation}
where $f$ is the velocity distribution function, $\bar{m}$ the mass of the nitrogen molecule, $v$ the velocity, $k_\mathrm{B}$ the Boltzmann constant, and $T$ the temperature.

The rotational energy of the gas molecule was sampled according to the Boltzmann distribution \citep{Hazenberg2023}
\begin{equation} \label{eq:mb_rot}
    \frac{N_i}{N} = \frac{g_i}{Z_\mathrm{rot}} \exp \left(\frac{E_\mathrm{rot,i}}{k_\mathrm{B} T}\right),
\end{equation}
with $N$ is the population, $N_i$ the number of particles in a state, $g_i$ the degeneracy of the energy state i, $Z_\mathrm{rot}$ the partition function and $E_\mathrm{rot,i}$ the rotational energy of the state $i$. Since quantum effects cannot be handled in MD simulations, this distribution is assumed to be continuous.

For the nitrogen molecule, it holds that $m_1 = m_2 = m$ and we assume that that initially $x_1 - x_2 = R$, $y_1 - y_2 = 0$ and $z_1 - z_2 = 0$. The velocity vector of the atoms can be described as
\begin{equation}
    v_i = v_{CoM,i} \pm dv_i,
\end{equation}
with $v_{CoM,i}$ the center of mass velocity derived from Equations \ref{eq:mb_vxy} and \ref{eq:mb_vz} and $dv_i$ the velocity of the atom with respect to the center of mass. The latter term could be determined from the rotational energy.

For linear molecules, like nitrogen, there can be no rotational motion around the line of atoms. Therefore, the rotational energy can be written as
\begin{equation}
    E_\mathrm{rot} = \frac{L_y^2 + L_z^2}{2I},
\end{equation}
with $L_i$ the angular momentum and $I$ the inertia tensor. The inertia tensor for linear diatomic molecule can be written as
\begin{equation}
    I = \mu R^2,
\end{equation}
with $\mu = \frac{m^2}{\bar{m}}$ the reduced mass.

The angular momentum can be written as
\begin{equation}
    L = \bar{m} \left(dr \times dv \right),
\end{equation}
with $dr$ the distance of the atom wrt to the center of mass. For a three dimensional case, the angular momentum becomes
\begin{equation}
    L = \begin{pmatrix}
L_x \\
L_y \\
L_z \\
\end{pmatrix} = \bar{m} \begin{pmatrix}
dy dv_z - dz dv_y \\
dz dv_x - dx dv_z \\
dx dv_y - dy dv_x \\
\end{pmatrix}.
\end{equation}
Substituting $dy = dz = 0$ and $L_x = 0$, we find that \begin{equation}
    dv_y = - \frac{\sqrt{I E_{rot}}}{\bar{m} dx},
\end{equation}
\begin{equation}
    dv_z = \frac{\sqrt{I E_{rot}}}{\bar{m} dx},
\end{equation}
with $dx$ equal to $1/2R$.
